# Supplementary material for: No evidence that natural selection has been less effective at removing deleterious mutations in Europeans than in West Africans
Source: arXiv:1402.4896 source file (2014-02-20)
Supplement: Supplementary file 1 [file Do_etal_SI_2_19_2014.pdf]

# Supplementary Materials

## No evidence that natural selection has been less effective at removing deleterious mutations in non-Africans than in West Africans


**Table of contents** 1

**Table S1 – Sample sizes in each dataset** 2

**Table S2 – Version of Table 1 for sites with a consistent allele among great apes** 3

**Table S3 – Expansion of Table 2 into PolyPhen-2 classes** 4-8

**Table S4 – Expected $R_{WestAfrica/Europe}$ for different models of demography** 9

**Table S5 – $R_{African/Non\text{-}African}$-statistic stratified by time depth of comparison** 10

**Table S6 – Biased Gene Conversion analysis for all population pairs** 11-12

**Table S7 – Key statistics as a function of allelic substitution patterns** 13

**Table S8 – $R^2_{X/Y}$-statistic for all population pairs** 14

**Table S9 – Parameters of simulated demographic models** 15

**Figure S1 – $R_{WestAfrica/Europe}$ for four demographic histories (simulations)** 16

**Supplementary References for Tables and Figures** 17

**Note S1 – Inferred distributions of selection coefficients for PolyPhen-2 classes** 18-27

**Note S2 – Proportion of non-synonymous sites is driven by neutral demography** 28-31

**Table S1: Sample sizes in each dataset**

| Dataset | Population | N |
|---|---|---|
| 24 diverse genomes[1] | Denisova | 1 |
| | Neanderthal | 1 |
| | Mbuti | 2 |
| | San | 2 |
| | Mandenka | 2 |
| | Yoruba | 2 |
| | Dinka | 2 |
| | Papuan | 2 |
| | Sardinian | 2 |
| | Dai | 2 |
| | Karitiana | 2 |
| | Han | 2 |
| | French | 2 |
| Lohmueller[2] | African American | 15 |
| | European American | 20 |
| 1000 Genomes[3] | ASW | 61 |
| | CEU | 85 |
| | CHB | 97 |
| | CHS | 100 |
| | CLM | 60 |
| | FIN | 93 |
| | GBR | 89 |
| | IBS | 14 |
| | JPT | 89 |
| | LWK | 96 |
| | MXL | 64 |
| | PUR | 55 |
| | TSI | 98 |
| | YRI | 88 |
| Exome Sequencing Project[4] | African American | 1,088 |
| | European American | 1,351 |

ASW: African Ancestry in Southwest US; CEU: Utah residents (CEPH) with Northern and Western European ancestry; CHB: Han Chinese in Beijing, China; CHS: Han Chinese South; CLM: Colombian in Medellin, Colombia; FIN: Finnish from Finland; GBR: British from England and Scotland (GBR); IBS: Iberian populations in Spain; JPT: Japanese in Tokyo, Japan; LWK: Luhya in Webuye, Kenya; MXL: Mexican Ancestry in Los Angeles, CA; MXL: Mexican Ancestry in Los Angeles, CA; PUR: Puerto Rican in Puerto Rico; TSI: Toscani in Italia: YRI: Yoruba in Ibadan, Nigeria.

## Table S2: Version of Table 1 for sites with a consistent allele among great apes

| | | | ***R:*** **Relative rate of lineage specific mutations** | | | | | $\boldsymbol{R^2}$**: Relative rate of homozygosity for lineage specific mutations** | | | | |
|---|---|---|---|---|---|---|---|---|---|---|---|---|
| **Data set** | **West Africans** | **Europeans** | ***R(synonymous)*** | ***R(All non-synonymous)*** | ***R(Benign)*** | ***R(Possibly damaging)*** | ***R(Probably damaging)*** | $R^2$***(synonymous)*** | $R^2$ ***(All non-synonymous)*** | $R^2$ ***(Benign)*** | $R^2$ ***(Possibly damaging)*** | $R^2$ ***(Probably damaging)*** |
| **24 deep genomes** | 4 | 4 | 1.011 (0.014) | 1.015 (0.015) | 1.015 (0.019) | 0.991 (0.039) | 1.038 (0.038) | 0.628 (0.015) | 0.626 (0.018) | 0.630 (0.021) | 0.570 (0.043) | 0.661 (0.052) |
| **Celera exomes** | 15 | 20 | 0.990 (0.012) | 1.012 (0.020) | 1.018 (0.023) | 1.009 (0.044) | 0.991 (0.043) | 0.599 (0.011) | 0.572 (0.051) | 0.585 (0.024) | 0.604 (0.054) | 0.572 (0.051) |
| **1KG exomes** | 88 | 85 | 1.001 (0.012) | 0.987 (0.013) | 0.992 (0.016) | 0.948 (0.029) | 1.003 (0.028) | 0.624 (0.013) | 0.616 (0.014) | 0.613 (0.017) | 0.575 (0.031) | 0.612 (0.035) |
| **ESP exomes** | 1,088 | 1,351 | 1.007 (0.011) | 0.999 (0.012) | 0.993 (0.014) | 0.984 (0.028) | 1.040 (0.030) | 0.603 (0.011) | 0.594 (0.014) | 0.585 (0.016) | 0.551 (0.025) | 0.628 (0.038) |

Notes: This is the same analysis as Table 1, restricting to sites where chimpanzee and at least one of gorilla and orangutan have an allele call and all of the great apes are consistent (data from the EPO six-way primate alignment). ±1 standard errors are from a Block Jackknife with 100 equally sized blocks. For the whole genomes, Yoruba+Mandenka represent West Africans, and French+Sardinian represent Europeans. For the 1000 Genomes Data (1KG), YRI represent West Africans and CEU Europeans. The Celera and ESP datasets use African Americans to represent people with West African ancestry.

## Table S3: Expansion of Table 2 into PolyPhen2 classes

*Table S3A– Synonymous mutations for all pairs of 24 deep genomes (bottom left) and 1000 Genomes populations (top right)*

| | | | IBS (Spanish) | GBR (British) | FIN (Finnish) | CEU (European) | JPT (Japanese) | CHS (Chinese) | CHB (Chinese) | PUR (Pu.Ric.) | MXL (Mexican) | CLM (Colomb.) | YRI (Nigerian) | LWK (Kenyan) | ASW (Afr. Am.) | 1KG |
|---|---|---|---|---|---|---|---|---|---|---|---|---|---|---|---|---|
| | | **TSI (98)** | 1.015 (0.004) | 1.002 (0.003) | 0.997 (0.004) | 0.999 (0.003) | 0.988 (0.008) | 0.994 (0.009) | 0.991 (0.008) | 1.002 (0.003) | 0.99 (0.005) | 0.991 (0.004) | 0.981 (0.009) | 0.973 (0.008) | 0.987 (0.007) | **TSI (Italian)** |
| | | | **IBS (14)** | 0.987 (0.004) | 0.982 (0.004) | 0.984 (0.004) | 0.974 (0.008) | 0.98 (0.008) | 0.977 (0.008) | 0.988 (0.005) | 0.976 (0.006) | 0.976 (0.005) | 0.97 (0.009) | 0.962 (0.009) | 0.975 (0.008) | **IBS (Spanish)** |
| | **Denis-ova (1)** | | | **GBR (89)** | 0.995 (0.003) | 0.997 (0.002) | 0.986 (0.008) | 0.992 (0.008) | 0.989 (0.008) | 1 (0.003) | 0.988 (0.005) | 0.989 (0.004) | 0.979 (0.009) | 0.972 (0.008) | 0.985 (0.007) | **GBR (British)** |
| **Neand-erthal** | n/a | **Neand-erthal(1)** | | | **FIN (93)** | 1.002 (0.003) | 0.991 (0.008) | 0.997 (0.008) | 0.994 (0.008) | 1.005 (0.004) | 0.993 (0.005) | 0.994 (0.004) | 0.983 (0.009) | 0.976 (0.009) | 0.99 (0.007) | **FIN (Finnish)** |
| **Dinka** | n/a | n/a | **Dinka (2)** | | | **CEU (85)** | 0.989 (0.008) | 0.994 (0.008) | 0.992 (0.008) | 1.003 (0.004) | 0.991 (0.005) | 0.991 (0.004) | 0.981 (0.009) | 0.974 (0.009) | 0.988 (0.008) | **CEU (Eur.)** |
| **Mand-enka** | n/a | n/a | 1.001 (0.013) | **Mand-enka (2)** | | | **JPT (89)** | 1.007 (0.003) | 1.004 (0.003) | 1.014 (0.007) | 1.003 (0.007) | 1.003 (0.007) | 0.99 (0.01) | 0.983 (0.009) | 0.997 (0.009) | **JPT (Japanese)** |
| **Mbuti** | n/a | n/a | 0.99 (0.013) | 0.993 (0.012) | **Mbuti (2)** | | | **CHS (100)** | 0.997 (0.002) | 1.008 (0.008) | 0.997 (0.007) | 0.997 (0.007) | 0.986 (0.01) | 0.978 (0.01) | 0.992 (0.009) | **CHS (Chinese)** |
| **San** | n/a | n/a | 0.979 (0.014) | 0.975 (0.014) | 0.982 (0.014) | **San (2)** | | | **CHB (97)** | 1.01 (0.007) | 0.999 (0.007) | 1 (0.007) | 0.988 (0.01) | 0.98 (0.009) | 0.994 (0.008) | **CHB (Chinese)** |
| **Yoruba** | n/a | n/a | 0.981 (0.013) | 0.981 (0.012) | 0.99 (0.011) | 1.004 (0.014) | **Yoruba (2)** | | | **PUR (55)** | 0.989 (0.004) | 0.989 (0.003) | 0.979 (0.008) | 0.972 (0.008) | 0.986 (0.007) | **PUR (Pu.Ric.)** |
| **Dai** | n/a | n/a | 0.969 (0.015) | 0.971 (0.014) | 0.978 (0.014) | 0.994 (0.014) | 0.988 (0.013) | **Dai (2)** | | | **MXL (64)** | 1 (0.004) | 0.988 (0.009) | 0.981 (0.008) | 0.995 (0.008) | **MXL (Mexican)** |
| **French** | n/a | n/a | 0.966 (0.013) | 0.971 (0.014) | 0.977 (0.014) | 0.991 (0.014) | 0.984 (0.012) | 0.995 (0.016) | **French (2)** | | | **CLM (60)** | 0.988 (0.008) | 0.98 (0.008) | 0.995 (0.007) | **CLM (Colomb.)** |
| **Han** | n/a | n/a | 0.99 (0.017) | 0.992 (0.014) | 0.996 (0.016) | 1.013 (0.015) | 1.009 (0.014) | 1.029 (0.015) | 1.028 (0.017) | **Han (2)** | | | **YRI (88)** | 0.992 (0.003) | 1.007 (0.003) | **YRI (Nigerian)** |
| **Karit-iana** | n/a | n/a | 0.983 (0.017) | 0.983 (0.015) | 0.986 (0.016) | 1.001 (0.016) | 0.994 (0.014) | 1.012 (0.015) | 1.02 (0.017) | 0.987 (0.018) | **Karitiana (2)** | | | **LWK (96)** | 1.015 (0.003) | **LWK (Kenyan)** |
| **Papuan** | n/a | n/a | 0.958 (0.015) | 0.962 (0.015) | 0.97 (0.015) | 0.982 (0.015) | 0.977 (0.013) | 0.985 (0.016) | 0.991 (0.016) | 0.959 (0.016) | 0.97 (0.016) | **Papuan (2)** | | | **ASW (61)** | |
| **Sard-inian** | n/a | n/a | 0.976 (0.013) | 0.972 (0.015) | 0.978 (0.015) | 0.996 (0.013) | 0.987 (0.013) | 1.004 (0.015) | 1.01 (0.013) | 0.978 (0.014) | 0.991 (0.016) | 1.018 (0.015) | **Sardinian (2)** | | | |
| **Deep genomes** | **Denis-ova** | **Neander-thal** | **Dinka** | **Mand-enka** | **Mbuti** | **San** | **Yoruba** | **Dai** | **French** | **Han** | **Karitiana** | **Papuan** | | | | |

Notes: ±1 standard errors (parentheses) are based on a Block Jackknife with 100 equally sized blocks. Highlighted numbers indicate P < 0.001.

* $R_{X/Y}$ ratios involving the ancient Denisova and Neanderthal samples are not shown as fewer mutations are expected for these than modern human lineages since divergence. Ratios are based on the accumulation of mutations observed in the population in the row divided by the accumulation of mutations observed in the population in the column. The number in parentheses indicates the number of samples per population.

*Table S3B– All non-synonymous mutations for all pairs of 24 deep genomes (bottom left) and 1000 Genomes populations (top right)*

| | | | **IBS (Spanish)** | **GBR (British)** | **FIN (Finnish)** | **CEU (European)** | **JPT (Japanese)** | **CHS (Chinese)** | **CHB (Chinese)** | **PUR (Pu.Ric.)** | **MXL (Mexican)** | **CLM (Colomb.)** | **YRI (Nigerian)** | **LWK (Kenyan)** | **ASW (Afr.Am.)** | **1KG** |
|---|---|---|---|---|---|---|---|---|---|---|---|---|---|---|---|---|
| | | **TSI (98)** | 1.026 (0.005) | 1.003 (0.003) | 1.003 (0.004) | 1 (0.003) | 0.998 (0.01) | 1.005 (0.011) | 1.001 (0.011) | 1.017 (0.004) | 1.014 (0.006) | 1.004 (0.005) | 1.005 (0.012) | 0.992 (0.011) | 1.013 (0.01) | **TSI (Italian)** |
| | | | **IBS (14)** | 0.978 (0.005) | 0.977 (0.005) | 0.974 (0.005) | 0.974 (0.011) | 0.981 (0.011) | 0.978 (0.011) | 0.993 (0.006) | 0.989 (0.008) | 0.979 (0.006) | 0.986 (0.012) | 0.972 (0.012) | 0.992 (0.01) | **IBS (Spanish)** |
| | **Denis-ova (1)** | | | **GBR (89)** | 0.999 (0.003) | 0.996 (0.002) | 0.995 (0.01) | 1.002 (0.011) | 0.998 (0.01) | 1.014 (0.005) | 1.011 (0.006) | 1.001 (0.005) | 1.003 (0.012) | 0.989 (0.011) | 1.01 (0.01) | **GBR (British)** |
| **Neand-erthal** | 0.875 (0.031) | **Neand-erthal (1)** | | | **FIN (93)** | 0.997 (0.003) | 0.995 (0.01) | 1.003 (0.011) | 0.999 (0.011) | 1.015 (0.005) | 1.011 (0.007) | 1.001 (0.005) | 1.003 (0.013) | 0.99 (0.012) | 1.011 (0.01) | **FIN (Finnish)** |
| **Dinka** | 0.862 (0.025) | 0.969 (0.031) | **Dinka (2)** | | | **CEU (85)** | 0.998 (0.011) | 1.005 (0.011) | 1.002 (0.011) | 1.018 (0.005) | 1.014 (0.007) | 1.004 (0.005) | 1.006 (0.013) | 0.992 (0.012) | 1.013 (0.01) | **CEU (European)** |
| **Mand-enka** | 0.865 (0.023) | 0.979 (0.028) | 1.014 (0.017) | **Mand-enka (2)** | | | **JPT (89)** | 1.008 (0.004) | 1.004 (0.003) | 1.019 (0.009) | 1.016 (0.008) | 1.006 (0.009) | 1.007 (0.013) | 0.993 (0.012) | 1.014 (0.011) | **JPT (Japanese)** |
| **Mbuti** | 0.884 (0.024) | 1.002 (0.026) | 1.03 (0.016) | 1.017 (0.016) | **Mbuti (2)** | | | **CHS (100)** | 0.996 (0.002) | 1.012 (0.009) | 1.009 (0.008) | 0.999 (0.009) | 1.001 (0.013) | 0.988 (0.012) | 1.008 (0.011) | **CHS (Chinese)** |
| **San** | 0.9 (0.026) | 1.009 (0.026) | 1.014 (0.016) | 1.004 (0.016) | 0.99 (0.017) | **San (2)** | | | **CHB (97)** | 1.015 (0.01) | 1.012 (0.008) | 1.002 (0.009) | 1.004 (0.013) | 0.99 (0.012) | 1.011 (0.011) | **CHB (Chinese)** |
| **Yoruba** | 0.863 (0.023) | 0.974 (0.025) | 0.99 (0.018) | 0.982 (0.016) | 0.965 (0.016) | 0.975 (0.017) | **Yoruba (2)** | | | **PUR (55)** | 0.996 (0.005) | 0.987 (0.003) | 0.992 (0.011) | 0.978 (0.01) | 0.998 (0.008) | **PUR (Pu.Ric.)** |
| **Dai** | 0.887 (0.027) | 1.01 (0.031) | 1.012 (0.019) | 1.001 (0.021) | 0.983 (0.018) | 0.999 (0.019) | 1.024 (0.019) | **Dai (2)** | | | **MXL (64)** | 0.99 (0.004) | 0.995 (0.011) | 0.981 (0.011) | 1.001 (0.009) | **MXL (Mexican)** |
| **French** | 0.874 (0.027) | 0.988 (0.031) | 0.992 (0.019) | 0.978 (0.02) | 0.961 (0.019) | 0.973 (0.019) | 0.997 (0.019) | 0.972 (0.018) | **French (2)** | | | **CLM (60)** | 1.002 (0.011) | 0.989 (0.01) | 1.01 (0.008) | **CLM (Colomb.)** |
| **Han** | 0.894 (0.028) | 1.014 (0.031) | 1.027 (0.018) | 1.016 (0.021) | 1 (0.019) | 1.018 (0.019) | 1.044 (0.02) | 1.021 (0.017) | 1.051 (0.019) | **Han (2)** | | | **YRI (88)** | 0.986 (0.004) | 1.007 (0.004) | **YRI (Nigerian)** |
| **Karitiana** | 0.862 (0.026) | 0.971 (0.028) | 0.97 (0.018) | 0.961 (0.019) | 0.943 (0.018) | 0.954 (0.018) | 0.975 (0.019) | 0.941 (0.019) | 0.97 (0.019) | 0.923 (0.018) | **Karitiana (2)** | | | **LWK (96)** | 1.27 (0.011) | **LWK (Kenyan)** |
| **Papuan** | 0.888 (0.026) | 1.011 (0.03) | 1.012 (0.021) | 0.999 (0.019) | 0.982 (0.02) | 0.997 (0.018) | 1.021 (0.02) | 1.002 (0.02) | 1.022 (0.018) | 0.976 (0.02) | 1.057 (0.021) | **Papuan (2)** | | | **ASW (61)** | |
| **Sardinian** | 0.894 (0.027) | 0.989 (0.028) | 0.997 (0.018) | 0.985 (0.019) | 0.967 (0.018) | 0.977 (0.018) | 1.006 (0.018) | 0.978 (0.017) | 1.004 (0.017) | 0.958 (0.017) | 1.035 (0.022) | 0.987 (0.018) | **Sardinian (2)** | | | |
| **Deep genomes** | **Denis-ova** | **Neand-erthal** | **Dinka** | **Mand-enka** | **Mbuti** | **San** | **Yoruba** | **Dai** | **French** | **Han** | **Karitiana** | **Papuan** | | | | |

Notes: ±1 standard errors (parentheses) are based on a Block Jackknife with 100 equally sized blocks. Highlighted numbers indicate P < 0.001.

* *R*-ratios computed using Denisova and Neanderthal are normalized by the number of synonymous sites on each lineage, to adjust for the fewer mutations in the ancient sample than on present-day human lineages since divergence (the *R´* statistic described in the main text). Ratios are based on the accumulation of mutations observed in the population in the row divided by the accumulation of mutations observed in the population shown in the column. The number in parentheses indicates the number of samples per population.

*Table S3C– PolyPhen2 "Benign" mutations for all pairs of 24 deep genomes (bottom left) and 1000 Genomes populations (top right)*

| | | | **IBS (Spanish)** | **GBR (British)** | **FIN (Finn)** | **CEU (Eur. Am.)** | **JPT (Jap.)** | **CHS (Chinese)** | **CHB (Chinese)** | **PUR (Pu.Ric.)** | **MXL (Mex)** | **CLM (Colom.)** | **YRI (Nigerian)** | **LWK (Kenyan)** | **ASW (Afr. Am.)** | **1KG** |
|---|---|---|---|---|---|---|---|---|---|---|---|---|---|---|---|---|
| | | **TSI (98)** | 1.02 (0.006) | 0.998 (0.004) | 0.995 (0.005) | 0.994 (0.004) | 1 (0.013) | 1.003 (0.014) | 1 (0.014) | 1.009 (0.005) | 1.007 (0.008) | 0.999 (0.006) | 0.996 (0.015) | 0.987 (0.014) | 1.006 (0.012) | **TSI (Italian)** |
| | | | **IBS (14)** | 0.979 (0.006) | 0.976 (0.007) | 0.974 (0.007) | 0.983 (0.014) | 0.985 (0.014) | 0.982 (0.014) | 0.991 (0.008) | 0.988 (0.01) | 0.981 (0.008) | 0.982 (0.015) | 0.972 (0.014) | 0.991 (0.012) | **IBS (Spanish)** |
| | **Denis-ova (1)** | | | **GBR (89)** | 0.996 (0.004) | 0.995 (0.003) | 1.002 (0.014) | 1.005 (0.014) | 1.001 (0.014) | 1.011 (0.006) | 1.008 (0.009) | 1.001 (0.006) | 0.997 (0.015) | 0.988 (0.014) | 1.008 (0.012) | **GBR (British)** |
| **Neand-erthal** | 0.939 (0.039) | **Neand-erthal (1)** | | | **FIN (93)** | 0.999 (0.004) | 1.005 (0.014) | 1.008 (0.014) | 1.004 (0.014) | 1.014 (0.007) | 1.012 (0.009) | 1.004 (0.007) | 1 (0.016) | 0.991 (0.015) | 1.011 (0.013) | **FIN (Finnish)** |
| **Dinka** | 0.911 (0.029) | 0.971 (0.032) | **Dinka (2)** | | | **CEU (85)** | 1.006 (0.014) | 1.009 (0.015) | 1.006 (0.014) | 1.015 (0.006) | 1.013 (0.009) | 1.005 (0.007) | 1.001 (0.015) | 0.992 (0.014) | 1.012 (0.012) | **CEU (European)** |
| **Mand-enka** | 0.906 (0.028) | 0.97 (0.03) | 0.996 (0.02) | **Mandenka (2)** | | | **JPT (89)** | 1.003 (0.005) | 0.999 (0.004) | 1.008 (0.012) | 1.006 (0.01) | 0.999 (0.011) | 0.996 (0.016) | 0.986 (0.015) | 1.006 (0.014) | **JPT (Japanese)** |
| **Mbuti** | 0.934 (0.031) | 1 (0.028) | 1.024 (0.021) | 1.022 (0.021) | **Mbuti (2)** | | | **CHS (100)** | 0.996 (0.003) | 1.005 (0.012) | 1.003 (0.01) | 0.995 (0.011) | 0.993 (0.016) | 0.984 (0.015) | 1.003 (0.014) | **CHS (Chinese)** |
| **San** | 0.946 (0.033) | 1.001 (0.029) | 1.006 (0.019) | 1.009 (0.02) | 0.988 (0.018) | **San (2)** | | | **CHB (97)** | 1.009 (0.012) | 1.007 (0.01) | 0.999 (0.011) | 0.996 (0.016) | 0.987 (0.015) | 1.007 (0.014) | **CHB (Chinese)** |
| **Yoruba** | 0.9 (0.029) | 0.963 (0.028) | 0.98 (0.021) | 0.987 (0.02) | 0.963 (0.019) | 0.976 (0.02) | **Yoruba (2)** | | | **PUR (55)** | 0.998 (0.006) | 0.99 (0.004) | 0.989 (0.013) | 0.98 (0.012) | 0.999 (0.01) | **PUR (Pu.Ric.)** |
| **Dai** | 0.925 (0.033) | 0.987 (0.032) | 0.984 (0.022) | 0.984 (0.024) | 0.965 (0.022) | 0.976 (0.023) | 1.001 (0.022) | **Dai (2)** | | | **MXL (64)** | 0.992 (0.005) | 0.991 (0.014) | 0.982 (0.013) | 1.001 (0.011) | **MXL (Mexican)** |
| **French** | 0.925 (0.033) | 0.987 (0.031) | 0.986 (0.023) | 0.987 (0.023) | 0.964 (0.024) | 0.978 (0.024) | 1.004 (0.023) | 0.998 (0.023) | **French (2)** | | | **CLM (60)** | 0.997 (0.013) | 0.988 (0.012) | 1.007 (0.01) | **CLM (Colomb.)** |
| **Han** | 0.932 (0.035) | 0.987 (0.033) | 0.998 (0.021) | 1 (0.024) | 0.981 (0.024) | 0.998 (0.023) | 1.022 (0.024) | 1.022 (0.02) | 1.021 (0.024) | **Han (2)** | | | **YRI (88)** | 0.99 (0.004) | 1.01 (0.005) | **YRI (Nigerian)** |
| **Karitiana** | 0.905 (0.032) | 0.954 (0.03) | 0.95 (0.023) | 0.954 (0.022) | 0.931 (0.022) | 0.942 (0.021) | 0.965 (0.023) | 0.954 (0.025) | 0.955 (0.024) | 0.935 (0.022) | **Karit-iana (2)** | | | **LWK (96)** | 1.02 (0.005) | **LWK (Kenyan)** |
| **Papuan** | 0.937 (0.032) | 1.001 (0.032) | 1 (0.024) | 1.002 (0.023) | 0.978 (0.024) | 0.992 (0.022) | 1.021 (0.023) | 1.023 (0.023) | 1.012 (0.022) | 0.999 (0.025) | 1.07 (0.028) | **Papuan (2)** | | | **ASW (61)** | |
| **Sard-inian** | 0.943 (0.034) | 0.981 (0.031) | 0.983 (0.022) | 0.992 (0.023) | 0.969 (0.023) | 0.979 (0.024) | 1.009 (0.022) | 1.003 (0.023) | 1.001 (0.022) | 0.987 (0.024) | 1.047 (0.029) | 0.991 (0.022) | **Sardinian (2)** | | | |
| **Deep genomes** | **Denis-ova** | **Neand-erthal** | **Dinka** | **Mandenka** | **Mbuti** | **San** | **Yoruba** | **Dai** | **French** | **Han** | **Karit-iana** | **Papuan** | | | | |

Notes: ±1 standard errors (parentheses) are based on a Block Jackknife with 100 equally sized blocks. Highlighted numbers indicate P < 0.001.

* *R*-ratios computed using Denisova and Neanderthal are normalized by the number of synonymous sites on each lineage, to adjust for the fewer mutations in the ancient sample than on present-day human lineages since divergence (the *R´* statistic described in the main text). Ratios are based on the accumulation of mutations observed in the population in the row divided by the accumulation of mutations observed in the population shown in the column. The number in parentheses indicates the number of samples per population.

*Table S3D – PolyPhen2 "Possibly damaging" mutations for all pairs of 24 deep genomes (bottom left) and 1000 Genomes populations (top right)*

| | | | **IBS (Spanish)** | **GBR (British)** | **FIN (Finnish)** | **CEU European** | **JPT Japanese** | **CHS Chinese** | **CHB Chinese** | **PUR Pu.Ric.** | **MXL Mexican** | **CLM Colom.** | **YRI Nigerian** | **LWK Kenyan** | **ASW Afr. Am.** | **1KG** |
|---|---|---|---|---|---|---|---|---|---|---|---|---|---|---|---|---|
| | | **TSI (98)** | 1.056 (0.013) | 1.024 (0.008) | 1.009 (0.012) | 1.013 (0.008) | 0.969 (0.025) | 0.985 (0.027) | 0.985 (0.026) | 1.045 (0.012) | 1.015 (0.018) | 1.006 (0.012) | 1.057 (0.031) | 1.026 (0.028) | 1.047 (0.024) | **TSI (Italian)** |
| | | | **IBS (14)** | 0.969 (0.012) | 0.955 (0.013) | 0.959 (0.012) | 0.921 (0.025) | 0.936 (0.026) | 0.935 (0.025) | 0.991 (0.013) | 0.963 (0.018) | 0.954 (0.013) | 1.014 (0.031) | 0.984 (0.028) | 1.002 (0.025) | **IBS (Spanish)** |
| | **Denisova (1)** | | | **GBR (89)** | 0.985 (0.009) | 0.989 (0.006) | 0.948 (0.025) | 0.963 (0.026) | 0.963 (0.025) | 1.021 (0.011) | 0.992 (0.018) | 0.983 (0.011) | 1.038 (0.031) | 1.007 (0.028) | 1.027 (0.024) | **GBR (British)** |
| **Neander-thal** | 0.830 (0.062) | **Neand-erthal(1)** | | | **FIN (93)** | 1.005 (0.01) | 0.961 (0.024) | 0.977 (0.026) | 0.977 (0.025) | 1.036 (0.012) | 1.007 (0.018) | 0.998 (0.012) | 1.05 (0.031) | 1.019 (0.028) | 1.04 (0.025) | **FIN (Finnish)** |
| **Dinka** | 0.808 (0.05) | 0.946 (0.065) | **Dinka (2)** | | | **CEU (85)** | 0.958 (0.026) | 0.973 (0.028) | 0.973 (0.027) | 1.031 (0.012) | 1.002 (0.018) | 0.993 (0.012) | 1.046 (0.031) | 1.015 (0.028) | 1.036 (0.024) | **CEU (European)** |
| **Mand-enka** | 0.842 (0.048) | 0.995 (0.06) | 1.075 (0.047) | **Mand-enka (2)** | | | **JPT (89)** | 1.019 (0.01) | 1.018 (0.009) | 1.075 (0.025) | 1.048 (0.023) | 1.037 (0.022) | 1.084 (0.033) | 1.052 (0.03) | 1.075 (0.029) | **JPT (Japanese)** |
| **Mbuti** | 0.848 (0.048) | 0.994 (0.062) | 1.043 (0.05) | 0.983 (0.044) | **Mbuti (2)** | | | **CHS (100)** | 0.999 (0.007) | 1.058 (0.025) | 1.03 (0.024) | 1.02 (0.022) | 1.069 (0.033) | 1.038 (0.03) | 1.06 (0.029) | **CHS (Chinese)** |
| **San** | 0.865 (0.047) | 1.021 (0.055) | 1.043 (0.044) | 0.982 (0.038) | 1.005 (0.042) | **San (2)** | | | **CHB (97)** | 1.058 (0.025) | 1.031 (0.023) | 1.021 (0.022) | 1.07 (0.033) | 1.038 (0.031) | 1.06 (0.029) | **CHB (Chinese)** |
| **Yoruba** | 0.844 (0.044) | 0.988 (0.054) | 1.017 (0.039) | 0.954 (0.036) | 0.979 (0.041) | 0.966 (0.035) | **Yoruba (2)** | | | **PUR (55)** | 0.972 (0.014) | 0.964 (0.009) | 1.021 (0.026) | 0.99 (0.024) | 1.009 (0.019) | **PUR (Pu.Ric.)** |
| **Dai** | 0.867 (0.057) | 1.048 (0.074) | 1.075 (0.048) | 1.022 (0.047) | 1.028 (0.052) | 1.049 (0.051) | 1.059 (0.048) | **Dai (2)** | | | **MXL (64)** | 0.991 (0.011) | 1.044 (0.029) | 1.014 (0.027) | 1.034 (0.023) | **MXL (Mexican)** |
| **French** | 0.82 (0.053) | 0.988 (0.065) | 1.013 (0.048) | 0.954 (0.044) | 0.968 (0.045) | 0.966 (0.044) | 0.994 (0.048) | 0.931 (0.042) | **French (2)** | | | **CLM (60)** | 1.052 (0.028) | 1.021 (0.025) | 1.041 (0.022) | **CLM (Colomb.)** |
| **Han** | 0.881 (0.057) | 1.069 (0.072) | 1.126 (0.049) | 1.055 (0.049) | 1.071 (0.05) | 1.078 (0.049) | 1.102 (0.051) | 1.061 (0.048) | 1.124 (0.051) | **Han (2)** | | | **YRI 88)** | 0.97 (0.008) | 0.988 (0.01) | **YRI (Nigerian)** |
| **Karitiana** | 0.848 (0.054) | 1.031 (0.069) | 1.068 (0.052) | 1.013 (0.048) | 1.008 (0.051) | 1.022 (0.049) | 1.034 (0.048) | 0.976 (0.048) | 1.04 (0.053) | 0.925 (0.051) | **Karit-iana (2)** | | | **LWK (96)** | 1.018 (0.011) | **LWK (Kenyan)** |
| **Papuan** | 0.868 (0.053) | 1.058 (0.07) | 1.071 (0.05) | 1.008 (0.046) | 1.019 (0.047) | 1.037 (0.05) | 1.05 (0.05) | 0.998 (0.049) | 1.068 (0.049) | 0.952 (0.045) | 1.012 (0.054) | **Papuan (2)** | | | **ASW (61)** | |
| **Sardinian** | 0.851 (0.054) | 1.004 (0.061) | 1.031 (0.051) | 0.968 (0.042) | 0.965 (0.043) | 0.975 (0.043) | 1.013 (0.046) | 0.937 (0.042) | 1.003 (0.037) | 0.881 (0.041) | 0.961 (0.05) | 0.946 (0.043) | **Sardinian (2)** | | | |
| **Deep genomes** | **Denis-ova** | **Neand-erthal** | **Dinka** | **Mand-enka** | **Mbuti** | **San** | **Yoruba** | **Dai** | **French** | **Han** | **Karit-iana** | **Papuan** | | | | |

Notes: ±1 standard errors (parentheses) are based on a Block Jackknife with 100 equally sized blocks. Highlighted numbers indicate P < 0.001.

* *R*-ratios computed using Denisova and Neanderthal are normalized by the number of synonymous sites on each lineage, to adjust for the fewer mutations in the ancient sample than on present-day human lineages since divergence (the *R´* statistic described in the main text). Ratios are based on the accumulation of mutations observed in the population in the row divided by the accumulation of mutations observed in the population shown in the column. The number in parentheses indicates the number of samples per population.

*Table S3E – PolyPhen2 "Probably damaging" mutations for all pairs of 24 deep genomes (bottom left) and 1000 Genomes populations (top right)*

| | | | | | | | | | | | | | | | | |
|---|---|---|---|---|---|---|---|---|---|---|---|---|---|---|---|---|
| | | | **IBS (Spanish)** | **GBR (British)** | **FIN (Finnish)** | **CEU European** | **JPT Japanese** | **CHS Chinese** | **CHB Chinese** | **PUR Pu.Ric.** | **MXL Mexican** | **CLM Colomb.** | **YRI Nigerian** | **LWK Kenyan** | **ASW Afr. Am.** | **1KG** |
| | | **TSI (98)** | 1.025 (0.013) | 1.004 (0.007) | 1.03 (0.009) | 1.012 (0.007) | 1.014 (0.025) | 1.029 (0.025) | 1.024 (0.025) | 1.026 (0.009) | 1.042 (0.018) | 1.022 (0.012) | 0.998 (0.026) | 0.981 (0.024) | 1.008 (0.021) | **TSI (Italian)** |
| | | | **IBS (14)** | 0.979 (0.013) | 1.005 (0.014) | 0.987 (0.013) | 0.991 (0.028) | 1.006 (0.028) | 1.001 (0.028) | 1.002 (0.014) | 1.018 (0.022) | 0.998 (0.016) | 0.978 (0.026) | 0.962 (0.025) | 0.987 (0.021) | **IBS (Spanish)** |
| | **Denis-ova (1)** | | | **GBR (89)** | 1.026 (0.008) | 1.008 (0.007) | 1.01 (0.026) | 1.026 (0.026) | 1.021 (0.026) | 1.023 (0.01) | 1.039 (0.019) | 1.018 (0.013) | 0.995 (0.027) | 0.978 (0.025) | 1.005 (0.022) | **GBR (British)** |
| **Neander-thal** | 0.695 (0.046) | **Neand-ertal(1)** | | | **FIN (93)** | 0.983 (0.008) | 0.986 (0.024) | 1.001 (0.025) | 0.996 (0.025) | 0.998 (0.011) | 1.014 (0.017) | 0.993 (0.012) | 0.975 (0.026) | 0.958 (0.024) | 0.984 (0.021) | **FIN (Finnish)** |
| **Dinka** | 0.724 (0.037) | 0.979 (0.058) | **Dinka (2)** | | | **CEU (85)** | 1.002 (0.025) | 1.018 (0.025) | 1.013 (0.025) | 1.015 (0.01) | 1.03 (0.018) | 1.01 (0.013) | 0.988 (0.026) | 0.971 (0.024) | 0.998 (0.021) | **CEU (European )** |
| **Mandenka** | 0.734 (0.036) | 1.004 (0.055) | 1.029 (0.042) | **Mand-enka (2)** | | | **JPT (89)** | 1.017 (0.009) | 1.012 (0.009) | 1.011 (0.023) | 1.028 (0.02) | 1.007 (0.022) | 0.986 (0.028) | 0.969 (0.026) | 0.995 (0.024) | **JPT (Japanese)** |
| **Mbuti** | 0.734 (0.034) | 1.014 (0.048) | 1.041 (0.041) | 1.026 (0.04) | **Mbuti (2)** | | | **CHS (100)** | 0.994 (0.007) | 0.996 (0.022) | 1.012 (0.02) | 0.991 (0.021) | 0.973 (0.028) | 0.957 (0.026) | 0.982 (0.024) | **CHS (Chinese)** |
| **San** | 0.759 (0.038) | 1.026 (0.056) | 1.024 (0.039) | 1.005 (0.04) | 0.98 (0.038) | **San (2)** | | | **CHB (97)** | 1.001 (0.022) | 1.017 (0.021) | 0.996 (0.021) | 0.978 (0.027) | 0.961 (0.026) | 0.986 (0.024) | **CHB (Chinese)** |
| **Yoruba** | 0.738 (0.036) | 1.004 (0.057) | 1.007 (0.035) | 0.985 (0.039) | 0.961 (0.036) | 0.975 (0.036) | **Yoruba (2)** | | | **PUR (55)** | 1.015 (0.014) | 0.995 (0.008) | 0.977 (0.022) | 0.96 (0.021) | 0.986 (0.017) | **PUR (Pu.Ric.)** |
| **Dai** | 0.765 (0.038) | 1.066 (0.063) | 1.075 (0.046) | 1.047 (0.046) | 1.013 (0.044) | 1.051 (0.04) | 1.085 (0.041) | **Dai (2)** | | | **MXL (64)** | 0.98 (0.012) | 0.964 (0.027) | 0.948 (0.026) | 0.972 (0.022) | **MXL (Mexican)** |
| **French** | 0.732 (0.037) | 0.993 (0.06) | 0.994 (0.045) | 0.959 (0.044) | 0.937 (0.044) | 0.957 (0.04) | 0.972 (0.039) | 0.908 (0.039) | **French (2)** | | | **CLM (60)** | 0.98 (0.024) | 0.963 (0.023) | 0.989 (0.019) | **CLM (Colomb.)** |
| **Han** | 0.762 (0.036) | 1.078 (0.057) | 1.061 (0.047) | 1.048 (0.048) | 1.013 (0.039) | 1.043 (0.041) | 1.08 (0.043) | 0.984 (0.041) | 1.11 (0.053) | **Han (2)** | | | **YRI (88)** | 0.983 (0.009) | 1.01 (0.009) | **YRI (Nigerian)** |
| **Karitiana** | 0.712 (0.041) | 0.988 (0.062) | 0.967 (0.047) | 0.938 (0.047) | 0.929 (0.045) | 0.938 (0.044) | 0.96 (0.044) | 0.861 (0.041) | 0.966 (0.046) | 0.875 (0.046) | **Karit-iana (2)** | | | **LWK (96)** | 1.027 (0.011) | **LWK (Kenyan)** |
| **Papuan** | 0.726 (0.038) | 1.008 (0.063) | 1.006 (0.052) | 0.974 (0.046) | 0.964 (0.044) | 0.979 (0.044) | 0.995 (0.048) | 0.924 (0.041) | 1.02 (0.048) | 0.911 (0.042) | 1.046 (0.053) | **Papuan (2)** | | | **ASW (61)** | |
| **Sardinian** | 0.75 (0.039) | 1.001 (0.057) | 1.02 (0.046) | 0.969 (0.043) | 0.958 (0.038) | 0.969 (0.043) | 0.988 (0.044) | 0.919 (0.041) | 1.014 (0.045) | 0.917 (0.04) | 1.052 (0.055) | 1.008 (0.048) | **Sardinian (2)** | | | |
| **Deep genomes** | **Denisova** | **Neander-thal** | **Dinka** | **Mand-enka** | **Mbuti** | **San** | **Yoruba** | **Dai** | **French** | **Han** | **Karit-iana** | **Papuan** | | | | |

Notes: ±1 standard errors (parentheses) are based on a Block Jackknife with 100 equally sized blocks. Highlighted numbers indicate P < 0.001.

* *R*-ratios computed using Denisova and Neanderthal are normalized by the number of synonymous sites on each lineage, to adjust for the fewer mutations in the ancient sample than on present-day human lineages since divergence (the *R´* statistic described in the main text). Ratios are based on the accumulation of mutations observed in the population in the row divided by the accumulation of mutations observed in the population shown in the column. The number in parentheses indicates the number of samples per population.

## Table S4: Expected $R_{WestAfrica/Europe}$ for different models of demography

| | $R^{All\ non-synionymous}$ | $R^{Benign}$ | $R_A^{Possibly\ damaging}$ | $R^{Probably\ damaging}$ |
|---|---|---|---|---|
| **Estimated percentage of sites in each of three selective coefficient bins** | | | | |
| **Percent of sites that are neutral** | 19% | 27% | 16% | 9% |
| **Percent of sites with weak selection coefficients: $s = -10^{-3}$** | 47% | 60% | 54% | 27% |
| **Percent of sites with strong selection coefficients: $s = -10^{-2}$** | 33% | 13% | 29% | 64% |
| **Model of history simulated** | | | | |
| **Tennessen[4]** | 0.989 | 0.990 | 0.985 | 0.988 |
| **Gravel[5]** | 0.987 | 0.988 | 0.984 | 0.986 |
| **Lohmueller[2]** | 0.992 | 0.993 | 0.989 | 0.991 |

Notes: As described in Note S1, we assume that selective coefficients take on only one of three values: $s = 0$ (“neutral”), $-10^{-3}$ (“weak”), and $-10^{-2}$ (“strong”), and then fit the density in each of these bits using site frequency spectrum data under the assumption of mutations all acting additively with no epistasis. In the bottom section of the table, we show the value of $R_{WestAfrica/Europe}$ expected for each demographic model and distribution of selective coefficients. The expected values are less than two standard errors from 1 (using the Block Jackknife standard errors from Table 1), indicating that do not expect much difference in the accumulation of deleterious mutations in Europeans than in West Africans.

**Table S5: $R_{African/Non\text{-}African}$-statistic stratified by time depth of comparison**

| | ***R(synonymous)*** | ***R(All non-synonymous)*** | ***R(Benign)*** | ***R(Possibly damaging)*** | ***R(Probably damaging)*** |
|---|---|---|---|---|---|
| **[0.0008-ancient)** | 1.046 (0.014) | 1.050 (0.017) | 1.063 (0.019) | 0.976 (0.059) | 1.025 (0.053) |
| **[0.0004-0.0008)** | 1.018 (0.022) | 1.026 (0.028) | 1.005 (0.046) | 1.028 (0.101) | 1.012 (0.057) |
| **[0-0.0004)** | 1.008 (0.033) | 1.009 (0.044) | 0.931 (0.061) | 1.017 (0.145) | 1.146 (0.093) |

Notes: ±1 standard errors are from a Block Jackknife with 20 equally sized contiguous blocks. For this analysis, we compare 4 sub-Saharan African to 6 non-African phased genomes. We restrict to sites that have a GATK genotype quality of ≥70, and that furthermore have a consistent genotype between GATK and samtools. The time stratification is in units of heterozygosity expected for segments of this time depth.

## Table S6: Biased gene conversion analysis for all population pairs

*Table S6A: Unnormalized $R_{X/Y}$ statistics: bottom left GC$\rightarrow$AT, top right AT$\rightarrow$GC*

| | Papuan | Karit-iana | Han | French | Dai | Yoruba | San | Mbuti | Mand-enka | Dinka | Denisova | Neander-thal | |
|---|---|---|---|---|---|---|---|---|---|---|---|---|---|
| **Sardin -ian (2)** | 0.994 (0.002) | 1.002 (0.002) | 0.984 (0.002) | 1.004 (0.001) | 0.99 (0.002) | 0.987 (0.002) | 0.975 (0.002) | 0.974 (0.002) | 0.979 (0.002) | 0.989 (0.002) | 1.104 (0.003) | 1.1 00 (0.003) | **Sardinian** |
| | **Papuan (2)** | 1.008 (0.002) | 0.991 (0.002) | 1.01 (0.002) | 0.996 (0.002) | 0.992 (0.002) | 0.979 (0.002) | 0.979 (0.002) | 0.985 (0.002) | 0.994 (0.002) | 1.110 (0.003) | 1.106 (0.003) | **Papuan** |
| | | **Kariti-ana (2)** | 0.981 (0.002) | 1.002 (0.002) | 0.987 (0.002) | 0.986 (0.002) | 0.973 (0.002) | 0.972 (0.002) | 0.978 (0.002) | 0.987 (0.002) | 1.103 (0.003) | 1.099 (0.003) | **Karitiana** |
| | | | **Han (2)** | 1.02 (0.002) | 1.006 (0.001) | 1 (0.002) | 0.988 (0.002) | 0.985 (0.002) | 0.992 (0.002) | 1.001 (0.002) | 1.112 (0.003) | 1.112 (0.003) | **Han** |
| | | | | **French (2)** | 0.986 (0.002) | 0.984 (0.002) | 0.972 (0.002) | 0.971 (0.002) | 0.977 (0.002) | 0.986 (0.002) | 1.102 (0.003) | 1.098 (0.003) | **French** |
| | | | | | **Dai (2)** | 0.996 (0.002) | 0.983 (0.002) | 0.981 (0.002) | 0.987 (0.002) | 0.997 (0.002) | 1.109 (0.003) | 1.108 (0.003) | **Dai** |
| | | | | | | **Yoruba (2)** | 0.986 (0.001) | 0.986 (0.001) | 0.992 (0.001) | 1.002 (0.001) | 1.116 (0.003) | 1.112 (0.002) | **Yoruba** |
| | | | | | | | **San (2)** | 1 (0.002) | 1.006 (0.002) | 1.015 (0.002) | 1.128 (0.003) | 1.125 (0.002) | **San** |
| | | | | | | | | **Mbuti (2)** | 1.007 (0.001) | 1.016 (0.001) | 1.127 (0.003) | 1.123 (0.003) | **Mbuti** |
| | | | | | | | | | **Mand-enka (2)** | 0.989 (0.002) | 1.121 (0.003) | 1.116 (0.003) | **Mandenka** |
| | | | | | | | | | | **Dinka (2)** | 1.112 (0.003) | 1.109 (0.003) | **Dinka** |
| | | | | | | | | | | | **Denisova (1)** | 0.998 (0.003) | **Denisova** |
| | | | | | | | | | | | | **Neander-thal (1)** | |

| | Neand-erthal | Denisova | Dinka | Mand-enka | Mbuti | San | Yoruba | Dai | French | Han | Karitiana | Papuan | |
|---|---|---|---|---|---|---|---|---|---|---|---|---|---|
| | **Neand-erthal (1)** | | | | | | | | | | | | |
| **Denisova** | 1.099 (0.003) | **Denisova (1)** | | | | | | | | | | | |
| **Dinka** | 1.057 (0.002) | 0.974 (0.002) | **Dinka (2)** | | | | | | | | | | |
| **Mandenka** | 1.065 (0.002) | 0.98 (0.002) | 1.01 (0.001) | **Mand-enka (2)** | | | | | | | | | |
| **Mbuti** | 1.069 (0.002) | 0.983 (0.002) | 1.013 (0.002) | 1.004 (0.001) | **Mbuti (2)** | | | | | | | | |
| **San** | 1.063 (0.002) | 0.978 (0.002) | 1.002 (0.001) | 0.994 (0.001) | 0.99 (0.001) | **San (2)** | | | | | | | |
| **Yoruba** | 1.054 (0.002) | 0.971 (0.002) | 0.994 (0.001) | 0.985 (0.001) | 0.981 (0.001) | 0.992 (0.001) | **Yoruba (2)** | | | | | | |
| **Dai** | 1.052 (0.002) | 0.969 (0.003) | 0.992 (0.002) | 0.984 (0.002) | 0.98 (0.002) | 0.991 (0.002) | 0.999 (0.002) | **Dai (2)** | | | | | |
| **French** | 1.047 (0.002) | 0.965 (0.002) | 0.986 (0.001) | 0.978 (0.001) | 0.975 (0.002) | 0.985 (0.002) | 0.992 (0.001) | 0.992 (0.002) | **French (2)** | | | | |
| **Han** | 1.057 (0.002) | 0.973 (0.003) | 0.998 (0.001) | 0.99 (0.001) | 0.986 (0.002) | 0.997 (0.002) | 1.006 (0.001) | 1.008 (0.001) | 1.016 (0.001) | **Han (2)** | | | |
| **Karitiana** | 1.046 (0.002) | 0.964 (0.003) | 0.986 (0.002) | 0.977 (0.002) | 0.974 (0.002) | 0.984 (0.002) | 0.992 (0.002) | 0.991 (0.002) | 0.999 (0.002) | 0.983 (0.002) | **Karitiana (2)** | | |
| **Papuan** | 1.051 (0.002) | 0.969 (0.003) | 0.992 (0.002) | 0.984 (0.002) | 0.98 (0.002) | 0.99 (0.001) | 0.998 (0.001) | 1 (0.002) | 1.007 (0.002) | 0.992 (0.002) | 1.008 (0.002) | **Papuan (2)** | |
| **Sardinian** | 1.05 (0.002) | 0.969 (0.002) | 0.992 (0.002) | 0.984 (0.001) | 0.981 (0.002) | 0.99 (0.002) | 0.998 (0.001) | 1 (0.002) | 1.008 (0.001) | 0.992 (0.001) | 1.008 (0.002) | 0.999 (0.002) | **Sardin -ian (2)** |

Notes: Ratios are based on the accumulation of mutations observed in the population in the row divided by the accumulation of mutations observed in the population in the column. The number in parentheses indicates the number of samples per population. ±1 standard errors (parentheses) are based on a Block Jackknife. Highlighted numbers indicate $P < 0.001$. We observe significant deviations from one in most pairwise comparisons. This could be due to different error rates across samples which are small but significant given the small standard errors, or different mutation rates across samples. We therefore correct for such systematic differences across samples in Table S6B by normalizing by the substitution rate differences at *G/C* and *A/T* sites, which are not subject to biased gene conversion.

*Table S6B: Normalized $R'_{X/Y}$ statistics: bottom left GC→AT, top right AT→GC*

| | | | | | | | | | | | | | | | | |
|---|---|---|---|---|---|---|---|---|---|---|---|---|---|---|---|---|
| | | | | **Papuan** | **Karit-iana** | **Han** | **French** | **Dai** | **Yoruba** | **San** | **Mbuti** | **Mand-enka** | **Dinka** | **Denisova** | **Neander-thal** | |
| | | | **Sardinian (2)** | 1.001 (0.003) | 1.002 (0.003) | 0.996 (0.003) | 0.994 (0.003) | 0.998 (0.003) | 0.994 (0.003) | 0.998 (0.002) | 0.996 (0.002) | 0.999 (0.003) | 0.997 (0.002) | 1.058 (0.003) | 1.009 (0.003) | **Sardinian** |
| | | | | **Papuan (2)** | 1.001 (0.003) | 0.995 (0.003) | 0.994 (0.003) | 0.996 (0.003) | 0.994 (0.003) | 0.997 (0.003) | 0.996 (0.003) | 0.998 (0.003) | 0.996 (0.003) | 1.059 (0.004) | 1.008 (0.003) | **Papuan** |
| | **Neander-thal (1)** | | | | **Karit-iana (2)** | 0.993 (0.003) | 0.992 (0.003) | 0.994 (0.003) | 0.993 (0.003) | 0.996 (0.003) | 0.994 (0.003) | 0.998 (0.003) | 0.995 (0.002) | 1.057 (0.004) | 1.008 (0.003) | **Karitiana** |
| **Denisova** | 1.041 (0.005) | **Denisova (1)** | | | | **Han (2)** | 0.999 (0.003) | 1.001 (0.003) | 0.998 (0.003) | 1.001 (0.003) | 1 (0.003) | 1.002 (0.003) | 1 (0.002) | 1.059 (0.004) | 1.011 (0.003) | **Han** |
| **Dinka** | 0.965 (0.003) | 0.928 (0.004) | **Dinka (2)** | | | | **French (2)** | 1.003 (0.003) | 0.999 (0.003) | 1.002 (0.002) | 1 (0.002) | 1.004 (0.002) | 1.001 (0.002) | 1.06 (0.003) | 1.01 (0.003) | **French** |
| **Mand-enka** | 0.963 (0.003) | 0.927 (0.004) | 0.998 (0.002) | **Mand-enka (2)** | | | | **Dai (2)** | 0.997 (0.003) | 1.001 (0.003) | 0.998 (0.002) | 1.001 (0.003) | 0.999 (0.002) | 1.059 (0.004) | 1.009 (0.003) | **Dai** |
| **Mbuti** | 0.964 (0.003) | 0.927 (0.004) | 0.997 (0.002) | 1 (0.003) | **Mbuti (2)** | | | | **Yoruba (2)** | 1.003 (0.003) | 1.002 (0.002) | 1.005 (0.002) | 1.004 (0.002) | 1.063 (0.003) | 1.013 (0.003) | **Yoruba** |
| **San** | 0.956 (0.003) | 0.92 (0.004) | 0.987 (0.002) | 0.99 (0.002) | 0.989 (0.003) | **San (2)** | | | | **San (2)** | 0.999 (0.002) | 1.002 (0.003) | 1 (0.002) | 1.061 (0.003) | 1.013 (0.003) | **San** |
| **Yoruba** | 0.961 (0.003) | 0.925 (0.004) | 0.995 (0.002) | 0.998 (0.002) | 0.997 (0.002) | 1.009 (0.002) | **Yoruba (2)** | | | | **Mbuti (2)** | 1.003 (0.002) | 1.001 (0.002) | 1.063 (0.003) | 1.013 (0.003) | **Mbuti** |
| **Dai** | 0.958 (0.003) | 0.925 (0.004) | 0.995 (0.002) | 0.998 (0.003) | 0.997 (0.003) | 1.009 (0.002) | 1.000 (0.002) | **Dai (2)** | | | | **Mand-enka (2)** | 0.998 (0.002) | 1.06 (0.003) | 1.01 (0.003) | **Mandenka** |
| **French** | 0.963 (0.003) | 0.929 (0.004) | 1.002 (0.002) | 1.005 (0.002) | 1.004 (0.003) | 1.015 (0.002) | 1.007 (0.002) | 1.009 (0.003) | **French (2)** | | | | **Dinka (2)** | 1.06 (0.003) | 1.012 (0.003) | **Dinka** |
| **Han** | 0.961 (0.003) | 0.927 (0.004) | 0.997 (0.002) | 1 (0.002) | 1 (0.003) | 1.01 (0.002) | 1.003 (0.003) | 1.003 (0.002) | 0.995 (0.003) | **Han (2)** | | | | **Denisova (1)** | 0.945 (0.004) | **Denisova** |
| **Karitiana** | 0.959 (0.003) | 0.924 (0.004) | 0.993 (0.003) | 0.997 (0.003) | 0.996 (0.003) | 1.007 (0.003) | 0.999 (0.003) | 0.998 (0.003) | 0.99 (0.003) | 0.995 (0.003) | **Karitiana (2)** | | | | **Neander-thal (1)** | |
| **Papuan** | 0.959 (0.003) | 0.924 (0.004) | 0.995 (0.002) | 0.997 (0.003) | 0.997 (0.003) | 1.008 (0.003) | 1.000 (0.003) | 0.999 (0.002) | 0.992 (0.003) | 0.997 (0.003) | 1.001 (0.003) | **Papuan (2)** | | | | |
| **Sardinian** | 0.963 (0.003) | 0.929 (0.004) | 1.001 (0.002) | 1.003 (0.002) | 1.003 (0.002) | 1.014 (0.002) | 1.006 (0.002) | 1.007 (0.003) | 0.998 (0.003) | 1.004 (0.003) | 1.008 (0.003) | 1.007 (0.003) | **Sardin-ian (2)** | | | |
| | **Neander-thal** | **Denisova** | **Dinka** | **Mand-enka** | **Mbuti** | **San** | **Yoruba** | **Dai** | **French** | **Han** | **Karitiana** | **Papuan** | | | | |

Notes: Ratios are based on the accumulation of mutations observed in the population in the row divided by the accumulation of mutations observed in the population in the column. The number in parentheses indicates the number of samples per population. ±1 standard errors (parentheses) are based on a Weighted Block Jackknife. Highlighted numbers indicate P < 0.001. Ratios are normalized by the sum of *A*→*T*, *T*→*A*, *C*→*G* and *G*→*C* mutations on each lineage, producing an $R'$ statistic that adjusts for differences in the rates of accumulations of mutations on different lineages since divergence. These differences can arise due to branch shortening in the archaic lineages, or to different rates of mutation in the different populations. By normalizing, we highlight any differences in rates that are above and beyond these processes.

## Table S7: Key statistics as a function of allelic substitution patterns

| Substitution type | Benign | Possibly damaging | Probably damaging | Non-synonymous |
|---|---|---|---|---|
| $R_{WestAfrica/Europe}$ | | | | |
| **C→T or G→A** | 0.981 (0.028) | 0.942 (0.059) | 0.978 (0.053) | 0.976 (0.023) |
| **T→C or A→G** | 1.035 (0.034) | 0.995 (0.082) | 0.941 (0.102) | 1.023 (0.029) |
| **A→C or T→G** | 1.016 (0.054) | 1.127 (0.112) | 1.183 (0.089) | 1.082 (0.042) |
| **C→A or G→T** | 1.001 (0.060) | 1.213 (0.127) | 1.113 (0.114) | 1.065 (0.051) |
| **A→T or T→A** | 1.017 (0.100) | 0.995 (0.188) | 0.927 (0.136) | 1.001 (0.076) |
| **C→G or G→C** | 0.971 (0.049) | 0.957 (0.082) | 1.078 (0.093) | 0.989 (0.038) |
| **All but C→T or G→A** | 1.018 (0.021) | 1.053 (0.051) | 1.073 (0.052) | 1.033 (0.017) |
| **All sites** | 1.002 (0.018) | 1.007 (0.040) | 1.031 (0.038) | 1.008 (0.015) |
| $R'_{WestAfrica/Europe}$ | | | | |
| **C→T or G→A** | 0.956 (0.030) | 0.918 (0.058) | 0.953 (0.049) | 0.951 (0.025) |
| **T→C or A→G** | 1.005 (0.043) | 0.966 (0.084) | 0.914 (0.099) | 0.993 (0.038) |
| **A→C or T→G** | 1.009 (0.080) | 1.118 (0.134) | 1.173 (0.134) | 1.074 (0.084) |
| **C→A or G→T** | 1.055 (0.087) | 1.278 (0.146) | 1.172 (0.145) | 1.122 (0.084) |
| **A→T or T→A** | 1.060 (0.143) | 1.039 (0.209) | 0.968 (0.158) | 1.044 (0.117) |
| **C→G or G→C** | 0.945 (0.064) | 0.931 (0.096) | 1.049 (0.106) | 0.962 (0.060) |
| **All but C→T or G→A** | 1.004 (0.029) | 1.038 (0.052) | 1.059 (0.051) | 1.019 (0.024) |
| **All sites** | 0.981 (0.022) | 0.986 (0.041) | 1.010 (0.037) | 0.987 (0.019) |
| $R'_{AllModern/Denisova}$ | | | | |
| **C→T or G→A** | 0.898 (0.035) | 0.828 (0.065) | 0.565 (0.033) | 0.812 (0.027) |
| **T→C or A→G** | 0.860 (0.046) | 0.904 (0.120) | 0.697 (0.091) | 0.851 (0.042) |
| **A→C or T→G** | 0.830 (0.119) | 0.725 (0.143) | 1.475 (0.313) | 0.908 (0.117) |
| **C→A or G→T** | 1.085 (0.127) | 0.789 (0.123) | 1.080 (0.189) | 1.026 (0.103) |
| **A→T or T→A** | 0.848 (0.162) | 0.919 (0.228) | 0.791 (0.227) | 0.857 (0.149) |
| **C→G or G→C** | 0.766 (0.075) | 0.799 (0.118) | 1.244 (0.207) | 0.833 (0.072) |
| **All but C→T or G→A** | 0.865 (0.039) | 0.810 (0.058) | 0.985 (0.070) | 0.872 (0.034) |
| **All sites** | 0.929 (0.029) | 0.870 (0.046) | 0.760 (0.035) | 0.889 (0.024) |
| $R'_{AllModern/Neanderthal}$ | | | | |
| **C→T or G→A** | 0.953 (0.040) | 0.994 (0.094) | 0.909 (0.059) | 0.953 (0.033) |
| **T→C or A→G** | 1.046 (0.056) | 1.053 (0.126) | 0.928 (0.156) | 1.038 (0.051) |
| **A→C or T→G** | 0.937 (0.105) | 1.132 (0.197) | 1.462 (0.283) | 1.085 (0.105) |
| **C→A or G→T** | 1.073 (0.125) | 0.991 (0.160) | 1.188 (0.201) | 1.086 (0.112) |
| **A→T or T→A** | 0.988 (0.214) | 0.786 (0.208) | 0.928 (0.224) | 0.944 (0.168) |
| **C→G or G→C** | 0.816 (0.070) | 1.099 (0.173) | 1.169 (0.185) | 0.919 (0.077) |
| **All but C→T or G→A** | 0.997 (0.037) | 1.074 (0.079) | 1.181 (0.092) | 1.037 (0.036) |
| **All sites** | 0.993 (0.026) | 1.065 (0.062) | 1.063 (0.054) | 1.015 (0.025) |
| $R'_{Denisova/Neanderthal}$ | | | | |
| **C→T or G→A** | 1.089 (0.060) | 1.210 (0.147) | 1.695 (0.160) | 1.215 (0.055) |
| **T→C or A→G** | 1.250 (0.098) | 1.072 (0.182) | 1.409 (0.277) | 1.244 (0.087) |
| **A→C or T→G** | 1.049 (0.184) | 1.594 (0.447) | 0.687 (0.201) | 1.083 (0.170) |
| **C→A or G→T** | 0.849 (0.128) | 1.188 (0.266) | 1.133 (0.251) | 0.966 (0.136) |
| **A→T or T→A** | 1.195 (0.275) | 0.913 (0.272) | 1.141 (0.387) | 1.135 (0.218) |
| **C→G or G→C** | 1.027 (0.138) | 1.368 (0.323) | 1.029 (0.204) | 1.091 (0.126) |
| **All but C→T or G→A** | 1.132 (0.068) | 1.290 (0.118) | 1.172 (0.140) | 1.164 (0.059) |
| **All sites** | 1.064 (0.044) | 1.198 (0.090) | 1.433 (0.096) | 1.141 (0.040) |

Notes: ±1 standard errors are from a Block Jackknife. Statistics computed using Denisova and Neanderthal are normalized by the number of synonymous sites on each lineage, to adjust for the fact that there has been less time for mutations to accumulate in the ancient lineages than present-day human lineages since divergence (the $R'$ statistic in the main text). Red highlighting indicates a nominal P < 0.001 for $R < 1$ or $R' < 1$, and green highlighting indicates a nominal P < 0.001 for $R > 1$ or $R' > 1$. These results document a significantly higher burden of deleterious mutations in Denisova than in present-day humans whether the analysis is performed over all sites or excluding C→T and G→A sites which are known to be subject to high rates of error in ancient DNA. There is no clear evidence of a higher load of deleterious mutations in Neanderthals compared with present-day humans.

## Table S8: $R^2$-statistic for all population pairs

| | | | | | | | | | | | |
|---|---|---|---|---|---|---|---|---|---|---|---|
| | **Dinka (2)** | | | | | | | | | | |
| **Mand-enka** | 0.927 (0.038) | **Mand-enka (2)** | | | | | | | | | |
| **Mbuti** | 0.956 (0.036) | 1.025 (0.038) | **Mbuti (2)** | | | | | | | | |
| **San** | 0.907 (0.032) | 0.962 (0.036) | 0.949 (0.036) | **San (2)** | | | | | | | |
| **Yoruba** | 0.92 (0.041) | 0.99 (0.04) | 0.969 (0.035) | 1.029 (0.038) | **Yoruba (2)** | | | | | | |
| **Dai** | 1.601 (0.066) | 1.684 (0.064) | 1.609 (0.065) | 1.681 (0.065) | 1.713 (0.071) | **Dai (2)** | | | | | |
| **French** | 1.448 (0.06) | 1.528 (0.066) | 1.454 (0.06) | 1.513 (0.064) | 1.541 (0.066) | 0.879 (0.034) | **French (2)** | | | | |
| **Han** | 1.608 (0.059) | 1.677 (0.07) | 1.605 (0.064) | 1.691 (0.068) | 1.702 (0.072) | 1.009 (0.036) | 1.142 (0.045) | **Han (2)** | | | |
| **Karitiana** | 2.141 (0.078) | 2.228 (0.082) | 2.091 (0.077) | 2.147 (0.079) | 2.239 (0.085) | 1.468 (0.054) | 1.619 (0.06) | 1.455 (0.052) | **Karitiana (2)** | | |
| **Papuan** | 1.879 (0.07) | 1.963 (0.078) | 1.867 (0.058) | 1.925 (0.064) | 1.975 (0.067) | 1.214 (0.048) | 1.358 (0.048) | 1.203 (0.049) | 0.866 (0.032) | **Papuan (2)** | |
| **Sardinian** | 1.524 (0.057) | 1.603 (0.063) | 1.522 (0.059) | 1.579 (0.059) | 1.612 (0.058) | 0.936 (0.034) | 1.064 (0.038) | 0.933 (0.034) | 0.655 (0.025) | 0.787 (0.029) | **Sardin-ian (2)** |
| | **Dinka** | **Mand-enka** | **Mbuti** | **San** | **Yoruba** | **Dai** | **French** | **Han** | **Karitiana** | **Papuan** | |

Notes: ±1 standard errors (parentheses) are based on a Block Jackknife. Highlighted numbers indicate $P < 0.001$.

* For all population pairs, we show the $R^2_{X/Y}$ statistic. Ratios are based on the expected rate in the population in the row divided by the expected rate in the population in the column. Number in parentheses indicates the samples per population.

## Table S9: Parameters of simulated demographic models

**Gravel**[5] [$\pi_{Eur}/\pi_{Afr}$=0.72 ; $F_{ST}$(Eur,Afr)=0.19]

| ***Time in gens.*** | **2*N*$_{Afr}$** | **2*N*$_{Eur}$** |
|---|---|---|
| 300000 ≤ t < 3880 | 28948 | |
| 3880 ≤ t < 5000 | 28948 | 3,722 |
| 5000 ≤ t ≤ 5921 | 28948 | $2064e^{.003858(t-5000)}$ |

**Simple bottleneck** [$\pi_{Eur}/\pi_{Afr}$=0.69 ; $F_{ST}$(Eur,Afr)=0.21]

| ***Time in gens.*** | **2*N*$_{Afr}$** | **2*N*$_{Eur}$** |
|---|---|---|
| 300000 ≤ t < 3880 | 28948 | |
| 3880 ≤ t < 4080 | 28948 | 500 |
| 4080 ≤ t ≤ 5921 | 28948 | 28948 |

**Tennessen**[4] [$\pi_{Eur}/\pi_{Afr}$=0.70 ; $F_{ST}$(Eur,Afr)=0.21]

| ***Time in gens.*** | **2*N*$_{Afr}$** | **2*N*$_{Eur}$** |
|---|---|---|
| 300000 ≤ t < 3880 | 28948 | |
| 3880 ≤ t < 5000 | 28,948 | 3,722 |
| 5000 ≤ t < 5716 | 28,948 | $2064e^{.00307(t-5000)}$ |
| 5716 ≤ t ≤ 5921 | $28948e^{.00166(t-5716)}$ | $18900e^{.00195(t-5716)}$ |

**Lohmueller**[2] [$\pi_{Eur}/\pi_{Afr}$=0.70 ; $F_{ST}$(Eur,Afr)=0.29]

| ***Time in gens.*** | **2*N*$_{Afr}$** | **2*N*$_{Eur}$** |
|---|---|---|
| 300000 ≤ t < 100002 | 15672 | |
| 100002 ≤ t < 101772 | 15556 | 11398 |
| 101772 ≤ t < 107706 | 51272 | 11398 |
| 107706 ≤ t ≤ 108580 | 51272 | 60060 |

Notes: All simulations use $\mu = 2\times10^{8}$ and burn in from generation 250,000 to 0. The switch from sampling every 100 to every 1 generations occurs at 1000 for the three models that end at time 5,921, and at +99,000 for the Lohmueller model[2]. Summary statistics at the end of the simulation are shown; $F_{ST}$ is computed based on all SNPs, resulting in a higher differentiation than calculations that restrict to common SNPs.

**Figure S1 – $R_{WestAfrica/Europe}$ for four demographic histories (simulations)**

We show the expected accumulation of deleterious mutation in West Africans compared with Europeans at the present. We explore a range of selection coefficients *s* and dominance coefficients *h*, for the four models of demographic history specified in Table S9. The left column gives the ratio and the right column the difference. We observe a greater accumulation of deleterious mutations in West Africans for recessively acting mutations (*h*=0), and a greater accumulation in Europeans for additively acting mutations (*h*=0.5).

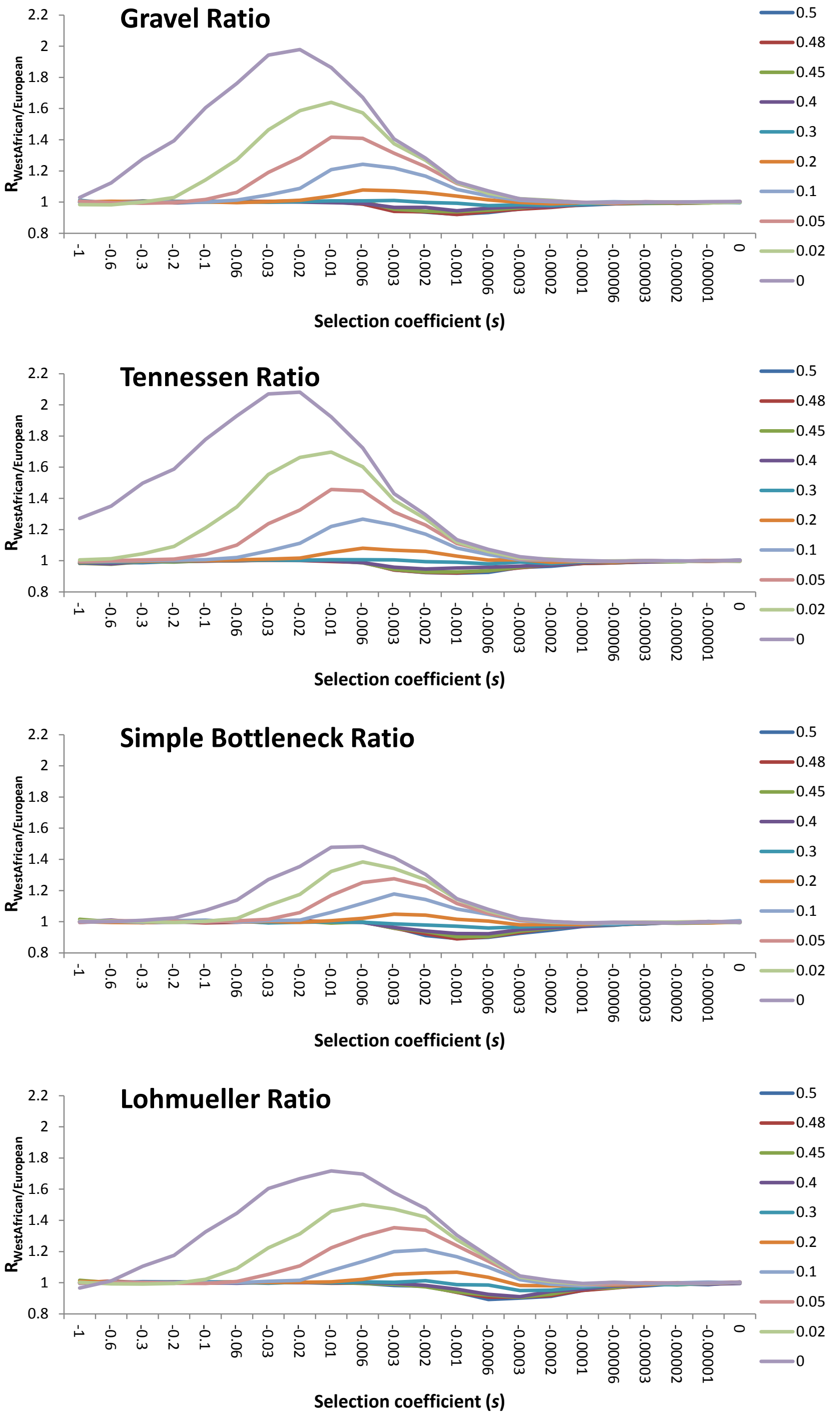

## Supplementary References


1. Meyer, M. *et al.* A high-coverage genome sequence from an archaic Denisovan individual. *Science* **338**, 222-6 (2012).
2. Lohmueller, K.E. *et al.* Proportionally more deleterious genetic variation in European than in African populations. *Nature* **451**, 994-7 (2008).
3. Abecasis, G.R. *et al.* An integrated map of genetic variation from 1,092 human genomes. *Nature* **491**, 56-65 (2012).
4. Tennessen, J.A. *et al.* Evolution and functional impact of rare coding variation from deep sequencing of human exomes. *Science* **337**, 64-9 (2012).
5. Gravel, S. *et al.* Demographic history and rare allele sharing among human populations. *Proc Natl Acad Sci U S A* **108**, 11983-8 (2011).
